# Supplementary material for: Transitions in Xenes between excitonic, topological and trivial insulator phases: influence of screening, band dispersion and external electric field
Source: arXiv:2301.08601 source file (2023-04-27)
Supplement: Supplementary file 1 [file Supplementary.pdf]

# Supplemental Material for:
# Transitions in Xenes between excitonic, topological and trivial insulator phases: influence of screening, band dispersion and external electric field

Olivia Pulci[1], Paola Gori[2], Davide Grassano[3], Marco D'Alessandro[4], and Friedhelm Bechstedt[51]

[11] *Department of Physics, and INFN, University of Rome Tor Vergata, Via della Ricerca Scientifica 1, I-00133 Rome, Italy*
[2] *Department of Industrial, Electronic and Mechanical Engineering, Roma Tre University, Via della Vasca Navale 79, I-00146 Rome, Italy*
[3] *Theory and Simulation of Materials (THEOS), École Polytechnique Federale de Lausanne, 1015 Lausanne, Switzerland*
[4] *Istituto di Struttura della Materia-CNR (ISM-CNR), Division of Ultrafast Processes in Materials (FLASHit), Via del Fosso del Cavaliere 100, 00133 Rome, Italy*
[5] *Institut für Festkörpertheorie und -optik, Friedrich-Schiller-Universität Jena, Max-Wien-Platz 1, 07743 Jena, Germany*

## I. XENES OPTICAL PROPERTIES ABOVE THE ABSORPTION EDGE

The normalized optical conductivities $Re\sigma(\omega)/\sigma_0$ of silicene, germanene, stanene, and plumbene are plotted in Fig. SM1 in a photon energy range near the absorption edge given by the SOC-induced fundamental gap $E_g$ and subsequent interband transitions. $\sigma(\omega)$ is directly related to the in-plane component of the frequency-dependent dielectric function $\epsilon_{\|}^{SL}(\omega)$ of a superlattice of sheets with a superlattice constant $L$ according to the formula [1–4]

$$\sigma(\omega) = -\frac{i\omega}{(4\pi)} L \left[\epsilon_{\|}^{SL}(\omega) - 1\right]. \tag{1}$$

Here $\epsilon_{\|}^{SL}(\omega)$ is computed from the DFT-PBE eigenfunctions and eigenvalues in the independent-particle approach. In the low-energy region, the *ab initio* spectra are compared with the analytically calculated lineshape [5, 6, 8]

$$Re\sigma(\omega) = \sigma_0 \left[1 + \left(\frac{E_g}{\hbar\omega}\right)^2\right] \theta(\hbar\omega - E_g) \tag{2}$$

with $\sigma_0 = \frac{e^2}{4\pi}$.

The numerically computed spectra show van Hove singularities in the intermediate energy range, which can be related to extrema and saddle points in the interband joint density of states [5, 6], while a step absorption edge appears at the gap energy $E_g$ in the low-energy limit. Such van Hove singularities have been experimentally observed for silicene on a Au substrate [7].

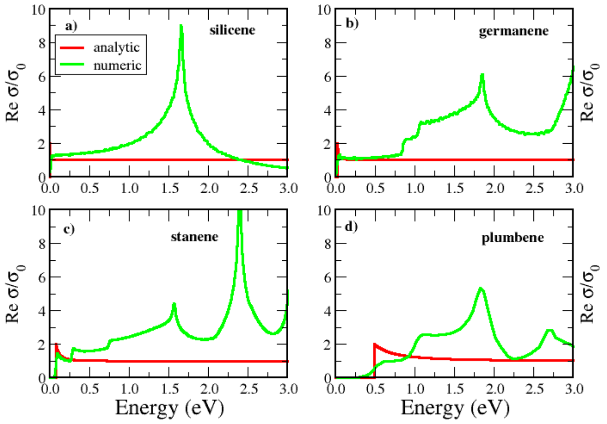


FIG. SM1. Green lines: Real part of the optical conductivity, renormalized to $\sigma_0 = e^2/4\hbar$, of (a) silicene, (b) germanene, (c) stanene, and (d) plumbene, calculated in the DFT-PBE framework with a small Lorentzian broadening parameter. For comparison, the analytic result of Eq. (2) (red lines) is displayed.

Close to the absorption edge, apart from a smearing due to Lorentzian broadening, the *ab initio* calculated spectra agree with the model lineshape in Eq. (2). Most important in the context discussed here is the absorption-free region $0 < \hbar\omega < E_g$ below the true absorption edge at $\hbar\omega = E_g$ in the independent-(quasi)particle treatment. It raises the question about what happens after inclusion of the excitonic effects. In a conventional semiconductor with $E_g > E_b$ the appearance of excitonic bound states with binding energy $E_b$ is expected. In the studied small gap systems, the Xenes, with reduced screening due to their low dimensionality, the occurrence of bound excitons with $E_b > E_g$, i.e., the formation of a spontaneously formed new electronic ground state, the EI phase, has to be investigated in a more rigorous way.

## II. BINDING ENERGY IN EMA UNDER EXTERNAL BIAS

By calculating the binding energy vs the applied external potential $U$ in the EMA approximation for the kinetic energy, and using the numerical values $\alpha_{2D}$(DFT)($U$), but the analytical continuation for finite $U$, we find a linear behavior of $E_b$, with $E_g > E_b$ in the full $U$ range.

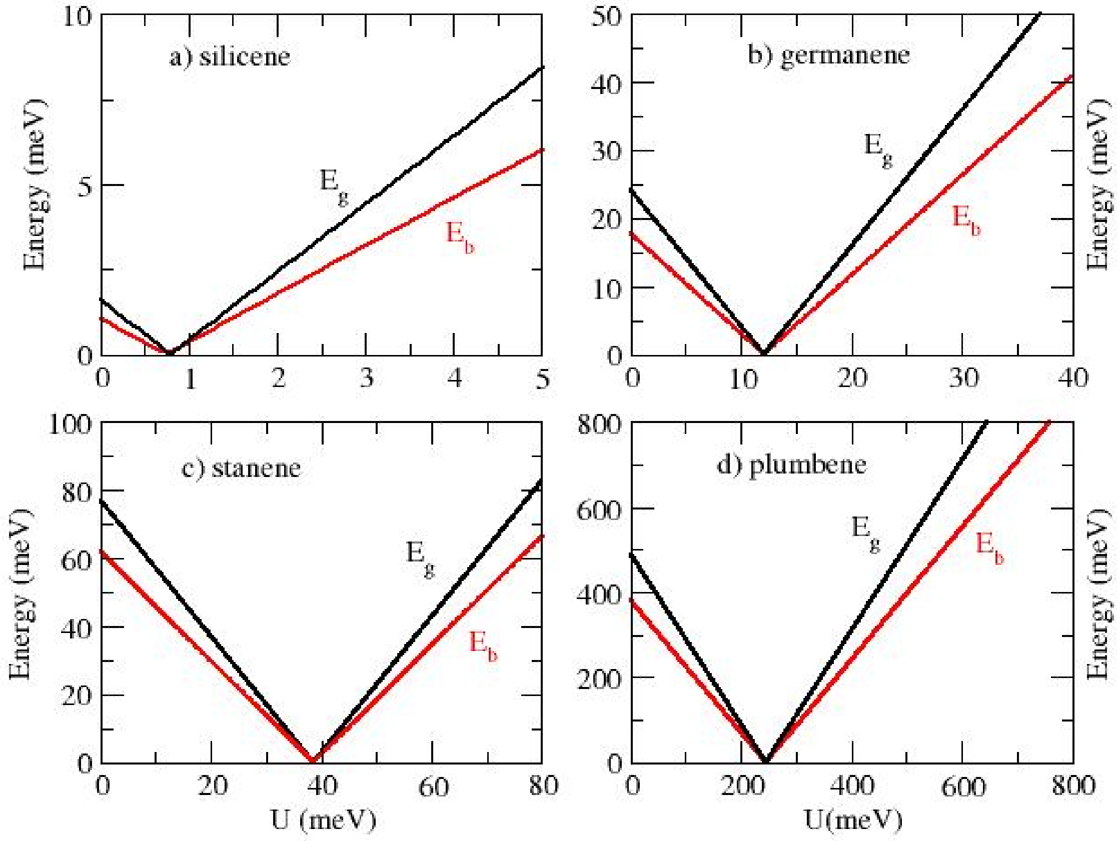


FIG. SM2. Exciton binding energy $E_b(U)$ (red), using the EMA for the kinetic energy, and direct gap $E_g(U)$ (black lines) at $K/K'$ as function of the applied potential energy difference $U$. The screening by $\alpha_{2D}$(DFT)($U$) has been used.

[1] L. Matthes, O. Pulci, and F. Bechstedt, Influence of out-of-plane response on optical properties of two-dimensional materials: First principles approach, Phys. Rev. B **94**, 205408 (2016).
[2] F. Bechstedt, L. Matthes, P. Gori, and O. Pulci, Silicene (Springer, Berlin, 2018) Chap. Optical Properties of Silicene and Related Materials from First Principles.
[3] C. Hogan, O. Pulci, P. Gori, F. Bechstedt, D. S. Martin, E. E. Barritt, A. Curcella, G. Prevot, and Y. Borensztein, Optical properties of silicene, Si/Ag(111), and Si/Ag(110), Phys. Rev. B **97**, 195407 (2018).
[4] L. Matthes, O. Pulci, and F. Bechstedt, Optical properties of two-dimensional honeycomb crystals graphene, silicene, germanene, and tinene from first principles, New Journal of Physics **16**, 105007 (2014).
[5] F. Bechstedt, L. Matthes, P. Gori, and O. Pulci, Infrared absorbance of silicene and germanene, Applied Physics Letters **100**, 261906 (2012).
[6] L. Matthes, P. Gori, O. Pulci, and F. Bechstedt, Universal infrared absorbance of two-dimensional honeycomb group-iv crystals, Phys. Rev. B **87**, 035438 (2013).
[7] J. Genser, D. Nazzari, V. Ritter, O. Bethge, K. Watanabe, T. Taniguchi, E. Bertagnolli, F. Bechstedt, and A. Lugstein, Nano Letters **21**, 5301 (2021).
[8] F. Bechstedt, P. Gori, and O. Pulci, Beyond graphene: Clean, hydrogenated and halogenated silicene, germanene, stanene, and plumbene, Progress in Surface Science **96**, 100615 (2021).
